# Supplementary material for: Loss of Hall Conductivity Quantization in a Non-Hermitian Quantum Anomalous Hall Insulator
Source: arXiv:1805.08892 ancillary file (2018-09-29)
Supplement: Supplementary file 1 [file Proximity_Effect_Supplement_v3.pdf]

# Supplemental Material for "Loss of Hall Conductivity Quantization in a Non-Hermitian Quantum Anomalous Hall Insulator"

Timothy M. Philip,[1,2,*] Mark R. Hirsbrunner,[2,3] and Matthew J. Gilbert[1,2,4]

[1] Department of Electrical and Computer Engineering, University of Illinois at Urbana-Champaign, Urbana, IL 61801, USA
[2] Micro and Nanotechnology Laboratory, University of Illinois, 208 N. Wright Street, Urbana IL 61801, USA
[3] Department of Physics, University of Illinois at Urbana-Champaign, Urbana, IL 61801, USA
[4] Department of Electrical Engineering, Stanford University, Stanford, California 94305, USA

## I. FERROMAGNET CONTACT SELF-ENERGY

The surface Green function of a semi-infinite, uniform lead is given by the equation[1]

$$[A(E) - H_{\text{hop}} g(E) H_{\text{hop}}^{\dagger}] g(E) = I, \tag{1}$$

where $A(E) = EI - H_{\text{on}}$, $E$ is the energy of interest, $I$ is the identity matrix, $H_{\text{on}}$ is the on-site Hamiltonian matrix for the surface of the contact, and $H_{\text{hop}}$ is the hopping matrix perpendicular to the contacting surface. Here, we derive the closed-form solution for the surface Green function assuming the matrices in Eq. (1) are 2×2 to match the dimensionality of the matrices for the Hamiltonian of the ferromagnet. We assume that the matrices in Eq. (1) have the form:

$$A(E) = \begin{bmatrix} a_{11} & 0 \\ 0 & a_{22} \end{bmatrix}, \qquad H_{\text{hop}} = \begin{bmatrix} -t & 0 \\ 0 & -t \end{bmatrix}, \text{ and } \qquad g(E) = \begin{bmatrix} g_{11} & g_{12} \\ g_{21} & g_{22} \end{bmatrix}. \tag{2}$$

We then solve for the components of the surface Green function using Eq. (1):

$$\left( \begin{bmatrix} a_{11} & 0 \\ 0 & a_{22} \end{bmatrix} - \begin{bmatrix} -t & 0 \\ 0 & -t \end{bmatrix} \begin{bmatrix} g_{11} & g_{12} \\ g_{21} & g_{22} \end{bmatrix} \begin{bmatrix} -t^* & 0 \\ 0 & -t^* \end{bmatrix} \right) \begin{bmatrix} g_{11} & g_{12} \\ g_{21} & g_{22} \end{bmatrix} = \begin{bmatrix} 1 & 0 \\ 0 & 1 \end{bmatrix} \tag{3}$$

$$\begin{bmatrix} (a_{11} - |t|^2 g_{11}) g_{11} - |t|^2 g_{12} g_{21} & (a_{11} - |t|^2 g_{11}) g_{12} - |t|^2 g_{12} g_{22} \\ - |t|^2 g_{12} g_{11} + (a_{22} - |t|^2 g_{22}) g_{21} & - |t|^2 g_{21} g_{12} + (a_{22} - |t|^2 g_{22}) g_{22}, \end{bmatrix} = \begin{bmatrix} 1 & 0 \\ 0 & 1 \end{bmatrix}. \tag{4}$$

The final matrix equation represents four coupled equations for the components of the surface Green function. We simultaneous solve the four equations and find the solutions:

$$g_{11} = \frac{a_{11} \pm \sqrt{a_{11}^2 - 4|t|^2}}{2|t|^2}, \tag{5}$$

$$g_{22} = \frac{a_{22} \pm \sqrt{a_{22}^2 - 4|t|^2}}{2|t|^2}, \tag{6}$$

$$g_{12} = g_{21} = 0. \tag{7}$$

Although this result is derived explicitly for the case where the matrices are 2×2, the result can be generalized for any diagonal $A$ matrix with diagonal matrix elements $a_{ii}$. The elements of the surface Green function are written as

$$g_{ii} = \frac{a_{ii} \pm \sqrt{a_{ii}^2 - 4|t|^2}}{2|t|^2}, \tag{8}$$

$$g_{ij(i \neq j)} = 0. \tag{9}$$

Once the surface Green function of the contact is found, the contact self-energies are given simply as

$$\Sigma_c(E) = H_{\text{coupling}}^{\dagger} g(E) H_{\text{coupling}}, \tag{10}$$

where $H_{\text{coupling}}$ is the coupling matrix between the system of interest and the contact.

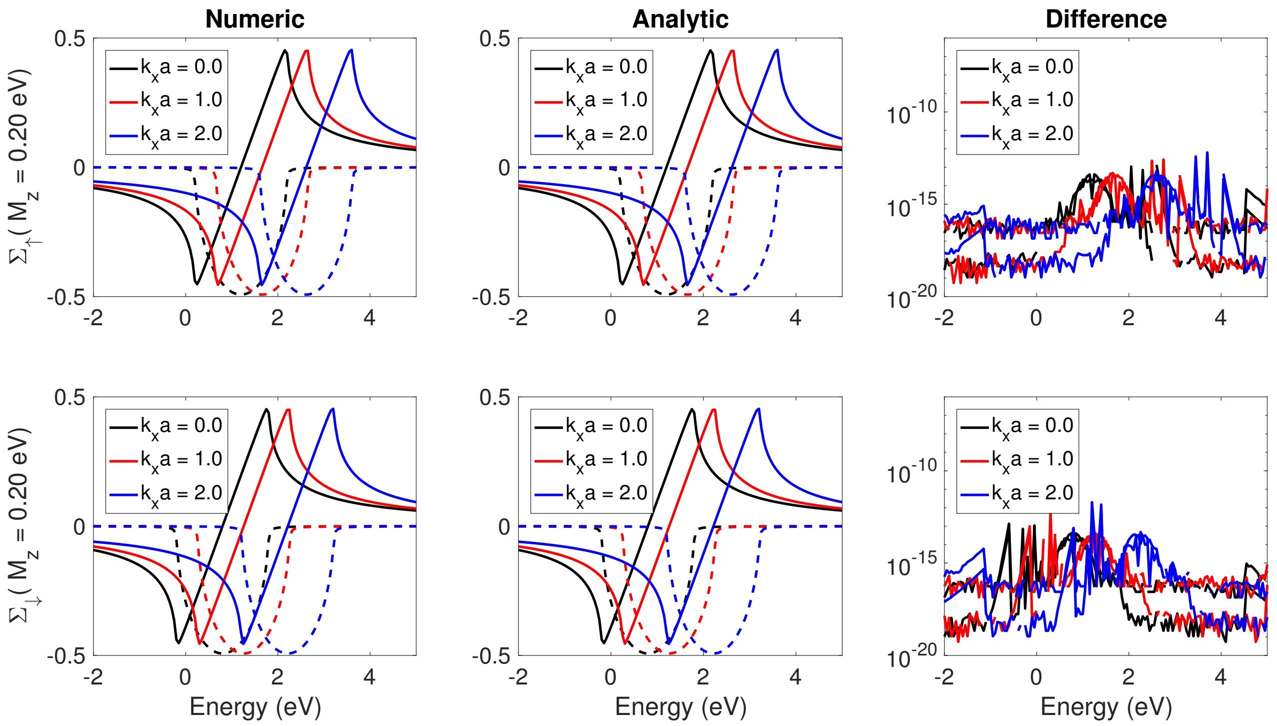


FIG. 1. Comparison of analytic ferromagnetic self-energy to numerical result at $k_x = 0, 1, 2$ and with $M_{\rm FM} = 0.2$ eV and in-plane dispersion $\epsilon(\mathbf{k}) = 2 - \cos k_x a - \cos k_y a$. The real part of the self-energy is given by the solid lines, while the imaginary is given by the dashed.

Using this closed-form solution for the contact self-energy of a semi-infinite contact, we apply it to the the tight-binding Hamiltonian given by Eq. (3) in the main text. This model Hamiltonian is parameterized with the matrices

$$H_{\rm on} = \epsilon(\mathbf{k})\sigma_0 + M_{\rm FM}\sigma_z, \tag{11}$$

$$H_{\rm hop} = -t_0\sigma_0, \tag{12}$$

where $\epsilon(\mathbf{k})$ is the dispersion of the energy bands in the in-plane direction, $M_{\rm FM}$ is the exchange coupling strength, and $\sigma_i$ are the spin Pauli matrices. We can write the surface Green function for a semi-infinite contact of this material as

$$g(E) = \begin{bmatrix} g_{11} & 0 \\ 0 & g_{22} \end{bmatrix} = \begin{bmatrix} g_\uparrow & 0 \\ 0 & g_\downarrow \end{bmatrix}, \tag{13}$$

where

$$g_\uparrow = \begin{cases} \frac{E-\epsilon(\mathbf{k})-M_{\rm FM}+\sqrt{(E-\epsilon(\mathbf{k})-M_{\rm FM})^2-4|t_0|^2}}{2|t_0|^2} & E \leq \epsilon(\mathbf{k}) + M_{\rm FM} \\ \frac{E-\epsilon(\mathbf{k})-M_{\rm FM}-\sqrt{(E-\epsilon(\mathbf{k})-M_{\rm FM})^2-4|t_0|^2}}{2|t_0|^2} & E > \epsilon(\mathbf{k}) + M_{\rm FM} \end{cases} \tag{14}$$

$$g_\downarrow = \begin{cases} \frac{E-\epsilon(\mathbf{k})+M_{\rm FM}+\sqrt{(E-\epsilon(\mathbf{k})+M_{\rm FM})^2-4|t_0|^2}}{2|t_0|^2} & E \leq \epsilon(\mathbf{k}) - M_{\rm FM} \\ \frac{E-\epsilon(\mathbf{k})+M_{\rm FM}-\sqrt{(E-\epsilon(\mathbf{k})+M_{\rm FM})^2-4|t_0|^2}}{2|t_0|^2} & E > \epsilon(\mathbf{k}) - M_{\rm FM} \end{cases} \tag{15}$$

The energy $E$ in these expressions must have a small, positive, imaginary component when evaluating this analytic formula. Otherwise, the imaginary part of this self-energy will have the wrong sign.

We assume that the coupling matrix between the TI surface state and the ferromagnet is given by $H_{\rm coupling} = -t_c\sigma_0$, resulting in the contact self-energy:

$$\Sigma_c(E) = |t_c|^2 \begin{bmatrix} g_\uparrow & 0 \\ 0 & g_\downarrow \end{bmatrix} = \begin{bmatrix} \Sigma_\uparrow & 0 \\ 0 & \Sigma_\downarrow \end{bmatrix}. \tag{16}$$

We verify this result in Fig. 1 by comparing the analytic expression derived here to the contact self-energy obtained through efficient numerical methods for the surface Green function.[2,3] We find that the difference between our analytic result and the numerical calculations are negligible.

## II. CALCULATION OF HALL CONDUCTIVITY FOR NON-ZERO BROADENING

Typical calculations of the DC Hall conductivity assume that broadening is negligible within the mass gap of the 2D Dirac Hamiltonian,[4,5] but the effective Hamiltonian we derive in Eq. (7) of the main text can have a large broadening contribution. Here we explicitly calculate the DC Hall conductivity assuming non-zero broadening for the massive 2D Dirac Hamiltonian

$$H_{\text{eff}} = -i\Gamma\sigma_0 + \alpha(\sigma_x k_y - \sigma_y k_x) - M\sigma_z. \tag{17}$$

To calculate the Hall conductivity for this effective Hamiltonian, we follow the methodology of Nunner *et al.* by using the Kubo-Streda formula.[5,6] It is useful to have the Green function, $G^r(E) = [(E + i0^+)\mathbb{I} - H_{\text{eff}}]^{-1}$ for this system, which is given as

$$G^r(E) = \frac{1}{(E+i\Gamma)^2 - M^2 - \alpha^2 k^2}\left[(E+i\Gamma)\sigma_0 + \alpha k_y\sigma_x - \alpha k_x \sigma_y - M\sigma_z\right], \tag{18}$$

$$= G^r_0\sigma_0 + G^r_x\sigma_x + G^r_y\sigma_y + G^r_z\sigma_z. \tag{19}$$

Here, the small imaginary part in the definition of the Green function, $0^+$, is absorbed into the much larger broadening term, $\Gamma$. The individual terms of this Green function can be written in a simpler form[5]

$$G^r_0 = \frac{1}{2}\left(G^r_+ + G^r_-\right), \tag{20}$$

$$G^r_x = \frac{\alpha k_y}{2\lambda_k}\left(G^r_+ - G^r_-\right), \tag{21}$$

$$G^r_y = -\frac{\alpha k_x}{2\lambda_k}\left(G^r_+ - G^r_-\right), \tag{22}$$

$$G^r_z = \frac{M}{2\lambda_k}\left(G^r_+ - G^r_-\right), \tag{23}$$

where

$$G^r_\pm = \frac{1}{E - E_{k\pm} + i\Gamma}, \tag{24}$$

$$E_{k\pm} = \pm\lambda_k, \tag{25}$$

$$\lambda_k = \sqrt{M^2 + \alpha^2 k^2}. \tag{26}$$

Using this analytic form of the Green function for the effective Hamiltonian, we explicitly evaluate the Kubo-Streda formula for the DC Hall conductivity given in Eqs. (9)-(11) of the main text.[4,5] One Fermi surface term, $\sigma^{\text{I}(b)}_{yx}$, identically vanishes, as the integrand is an odd function of momentum:

$$\sigma^{\text{I}(b)}_{yx} = -\frac{e^2\hbar}{4\pi V}\text{tr}\left\langle v_y G^r(\epsilon_F) v_x G^r(\epsilon_F) + v_y G^a(\epsilon_F) v_x G^a(\epsilon_F)\right\rangle \tag{27}$$

$$= -\frac{e^2}{4\pi\hbar}\int\frac{d^2k}{(2\pi)^2}\frac{\alpha^4}{\lambda_k^2}k_x k_y\left[(G^a_- - G^a_+)^2 + (G^r_- - G^r_+)^2\right] \tag{28}$$

$$= -\frac{e^2}{4\pi\hbar}\int_{-\infty}^{\infty}\int_{-\infty}^{\infty}\frac{dk_x dk_y}{(2\pi)^2}\frac{\alpha^4}{\lambda_k^2}k_x k_y\left[(G^a_- - G^a_+)^2 + (G^r_- - G^r_+)^2\right] \tag{29}$$

$$\sigma^{\text{I}(b)}_{yx} = 0. \tag{30}$$

The Fermi surface contribution to the Hall conductivity is then fully captured by $\sigma^{\text{I}(a)}_{yx}$. Here, we derive this contribution in the presence of finite broadening.

$$\sigma^{\text{I}(a)}_{yx} = \frac{e^2\hbar}{2\pi V}\text{tr}\left\langle v_y G^r(\epsilon_F) v_x G^a(\epsilon_F)\right\rangle \tag{31}$$

$$= \frac{e^2\hbar}{2\pi}\int\frac{d^2k}{(2\pi)^2}\text{tr}\left\langle v_y G^r(\epsilon_F) v_x G^a(\epsilon_F)\right\rangle \tag{32}$$

$$= \frac{e^2}{2\pi\hbar}\int \frac{d^2k}{(2\pi)^2}\frac{\alpha^2}{\lambda_k^2}\left[\alpha^2 k_x k_y (G_+^a - G_-^a)(G_+^r - G_-^r) + iM\lambda_k (G_+^a G_-^r - G_-^a G_+^r)\right] \tag{33}$$

$$= -\frac{e^2}{h}\frac{4\alpha^2 M\Gamma}{2\pi}\int_0^\infty dk \frac{k}{\left(\Gamma^2+\lambda_k^2\right)^2 + \epsilon_F^4 + 2\epsilon_F^2(\Gamma-\lambda_k)(\Gamma+\lambda_k)}. \tag{34}$$

Using the relationship $d\lambda_k/dk = \alpha^2 k/\lambda_k$:

$$\sigma_{yx}^{\mathrm{I}(a)} = -\frac{e^2}{h}\frac{4M\Gamma}{2\pi}\int_M^\infty d\lambda_k \frac{\lambda_k}{\left(\Gamma^2+\lambda_k^2\right)^2 + \epsilon_F^4 + 2\epsilon_F^2(\Gamma-\lambda_k)(\Gamma+\lambda_k)} \tag{35}$$

$$= -\frac{e^2}{h}\frac{M}{\epsilon_F 2\pi}\left[\frac{\pi}{2} - \arctan\left(\frac{\Gamma^2+M^2-\epsilon_F^2}{2\epsilon_F\Gamma}\right)\right]. \tag{36}$$

Care must be taken when taking the $\epsilon_F \to 0$ of this expression since the prefactor diverges. To appropraitely take this limit, one must recognize that the term within the brackets also approaches zero, so one must account for this using L'Hôpital's rule. Alternatively, one can take the limit of $\epsilon_F \to 0$ before integrating Eq. (35):

$$\lim_{\epsilon_F\to 0}\sigma_{yx}^{\mathrm{I}(a)} = -\frac{e^2}{h}\frac{4M\Gamma}{2\pi}\int_M^\infty d\lambda_k \frac{\lambda_k}{\left(\Gamma^2+\lambda_k^2\right)^2} \tag{37}$$

$$= -\frac{e^2}{h}\frac{M}{\pi}\frac{\Gamma}{\Gamma^2+M^2} \tag{38}$$

In the limit $\Gamma \to 0$, the Fermi surface contribution to the Hall conductivity, $\sigma_{yx}^{\mathrm{I}(a)}$, vanishes within the gap, since there are no states present to carry the current. When the broadening is finite, however, the Fermi surface contribution is nonzero since the Lorentzian tails of the broadened states now cross the Fermi surface.

Next, we now calculate the Fermi sea contribution to the Hall conductivity, $\sigma_{yx}^{\mathrm{II}}$, which is the source of the quantum anomalous Hall effect (QAHE). Typically, calculation of this term assumes the clean limit where $\Gamma \to 0$, which is a useful and accurate approximation when the broadening comes from disorder in the sample and is small compared to the mass gap. In the case of a proximity-coupled metal, $\Gamma$ can be on the order of the mass gap, so we explicitly calculate $\sigma_{yx}^{\mathrm{II}}$ with finite $\Gamma$. We start with the expression in Eq. (11) of the main text:

$$\sigma_{yx}^{\mathrm{II}} = \frac{e^2\hbar}{4\pi V}\int_{-\infty}^\infty d\epsilon\, f(\epsilon)\mathrm{tr}\left\langle v_y G^r(\epsilon) v_x \frac{dG^r(\epsilon)}{d\epsilon} - v_y\frac{dG^r(\epsilon)}{d\epsilon}v_x G^r(\epsilon) \right. \\ \left. - v_y G^a(\epsilon) v_x \frac{dG^a(\epsilon)}{d\epsilon} + v_y \frac{dG^a(\epsilon)}{d\epsilon} v_x G^a(\epsilon)\right\rangle. \tag{39}$$

After substituting in the expression for the Green function in Eqs. (19)-(23) and the velocity operators $v_x = -\frac{\alpha}{\hbar}\sigma_y$ and $v_y = \frac{\alpha}{\hbar}\sigma_x$, we can simplify this equation to

$$\sigma_{yx}^{\mathrm{II}} = -\frac{e^2}{4\pi\hbar}\int\frac{d^2k}{(2\pi)^2}\left(\frac{2i\alpha^2 M}{\lambda_k}\right)\int_{-\infty}^\infty d\epsilon\, f(\epsilon)\left(G_+^r(\epsilon)\frac{dG_-^r(\epsilon)}{d\epsilon} - G_-^r(\epsilon)\frac{dG_+^r(\epsilon)}{d\epsilon}\right. \\ \left. - G_+^a(\epsilon)\frac{dG_-^a(\epsilon)}{d\epsilon} + G_-^a(\epsilon)\frac{dG_+^a(\epsilon)}{d\epsilon}\right). \tag{40}$$

Here, we have also converted the trace to an integral over momentum space. By recognizing that $dG_\pm^{r/a}/d\epsilon = -(G_\pm^{r/a})^2$, we can further simplify this expression for $\sigma_{yx}^{\mathrm{II}}$:

$$\sigma_{yx}^{\mathrm{II}} = -\frac{e^2}{2h}\int\frac{d^2k}{(2\pi)^2}\left(\frac{2i\alpha^2 M}{\lambda_k}\right)\int_{-\infty}^\infty d\epsilon\, f(\epsilon)\left(-G_+^r(\epsilon)[G_-^r(\epsilon)]^2 + G_-^r(\epsilon)[G_+^r(\epsilon)]^2\right. \\ \left. + G_+^a(\epsilon)[G_-^a(\epsilon)]^2 - G_-^a(\epsilon)[G_+^a(\epsilon)]^2\right). \tag{41}$$

$$= \frac{e^2}{h}2\alpha^2 M\int\frac{d^2k}{(2\pi)^2}\frac{1}{\lambda_k}\int_{-\infty}^\infty d\epsilon\, f(\epsilon)\,\mathrm{Im}\left[G_+^r G_-^r\left(G_+^r - G_-^r\right)\right] \tag{42}$$

$$= \frac{e^2}{h}2\alpha^2 M\int\frac{d^2k}{(2\pi)^2}\frac{1}{\lambda_k}\int_{-\infty}^\infty d\epsilon\, f(\epsilon)\,\mathrm{Im}\left[\frac{2\lambda_k}{(E-E_{k+}+i\Gamma)^2(E-E_{k-}+i\Gamma)^2}\right] \tag{43}$$

$$= \frac{e^2}{h}2\alpha^2 M\int_0^{2\pi}\frac{d\theta}{(2\pi)^2}\int_0^\infty k\,dk\,\frac{1}{\lambda_k}\int_{-\infty}^\infty d\epsilon\, f(\epsilon)\,\mathrm{Im}\left[\frac{2\lambda_k}{(E-E_{k+}+i\Gamma)^2(E-E_{k-}+i\Gamma)^2}\right] \tag{44}$$

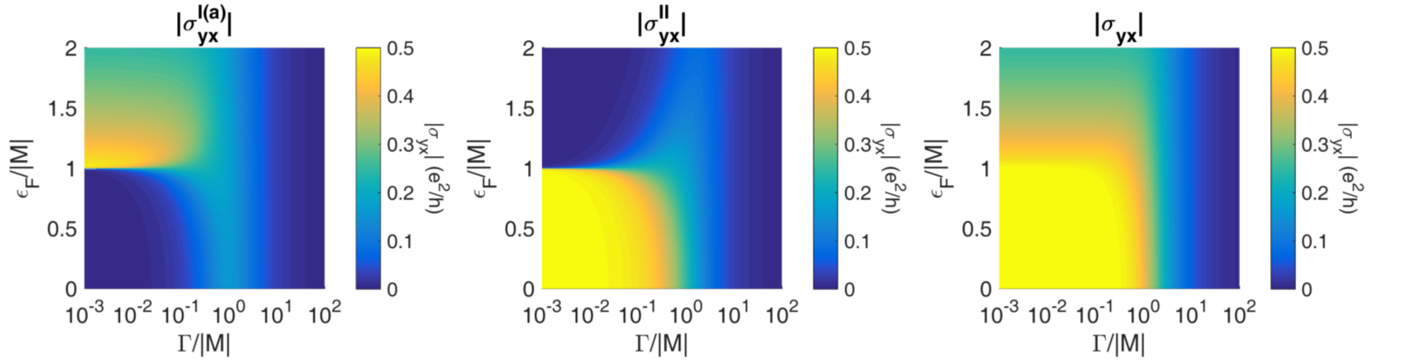


FIG. 2. The magnitudes of the Fermi surface contribution to the Hall conductivity, $\sigma_{yx}^{\mathrm{I(a)}}$, Fermi sea contribution to the Hall conductivity $\sigma_{yx}^{\mathrm{II}}$, and total Hall conductivity, $\sigma_{yx} = \sigma_{yx}^{\mathrm{I(a)}} + \sigma_{yx}^{\mathrm{II}}$ as functions of both the Fermi energy, $\epsilon_F$ and the non-Hermitian broadening, $\Gamma$.

$$= \frac{e^2}{h}\frac{2\alpha^2 M}{\pi}\int_0^\infty k\,dk\int_{-\infty}^{\infty} d\epsilon\, f(\epsilon)\,\mathrm{Im}\left[\frac{1}{(E-E_{k+}+i\Gamma)^2(E-E_{k-}+i\Gamma)^2}\right]. \tag{45}$$

We take the zero temperature limit, which gives us the expression:

$$\sigma_{yx}^{\mathrm{II}} = \frac{e^2}{h}\frac{2\alpha^2 M}{\pi}\int_0^\infty k\,dk\int_{-\infty}^{\epsilon_F} d\epsilon\,\mathrm{Im}\left[\frac{1}{(E-E_{k+}+i\Gamma)^2(E-E_{k-}+i\Gamma)^2}\right] \tag{46}$$

$$= \frac{e^2}{h}\frac{2\alpha^2 M}{\pi}\int_0^\infty k\,dk\int_{-\infty}^{\epsilon_F} d\epsilon\,\frac{4\Gamma\epsilon\left(\Gamma^2+\lambda_k^2-\epsilon^2\right)}{\left(\Gamma^2+(\epsilon-\lambda_k)^2\right)^2\left(\Gamma^2+(\lambda_k+\epsilon)^2\right)^2} \tag{47}$$

$$= \frac{e^2}{h}\frac{\alpha^2 M}{2\pi}\int_0^\infty k\,dk\left[\frac{\Gamma}{\lambda_k^2(\Gamma^2+(\epsilon_F-\lambda_k)^2)}+\frac{\Gamma}{\lambda_k^2(\Gamma^2+(\epsilon_F+\lambda_k)^2)}+\frac{1}{\lambda_k^3}\arctan\left(\frac{\epsilon_F^2+\Gamma^2-\lambda_k^2}{2\Gamma\lambda_k}\right)-\frac{\pi}{2\lambda_k^3}\right]. \tag{48}$$

Again making use of the fact that $d\lambda_k/dk = \alpha^2 k/\lambda_k$, we use a change of variable to perform the integration:

$$\sigma_{yx}^{\mathrm{II}} = \frac{e^2}{h}\frac{M}{2\pi}\int_{|M|}^\infty d\lambda_k\left[\frac{\Gamma}{\lambda_k(\Gamma^2+(\epsilon_F-\lambda_k)^2)}+\frac{\Gamma}{\lambda_k(\Gamma^2+(\epsilon_F+\lambda_k)^2)}+\frac{1}{\lambda_k^2}\arctan\left(\frac{\epsilon_F^2+\Gamma^2-\lambda_k^2}{2\Gamma\lambda_k}\right)-\frac{\pi}{2\lambda_k^2}\right] \tag{49}$$

$$= -\frac{e^2}{h}\frac{\mathrm{sgn}\,M}{2\pi}\left[\frac{\pi}{2}-\arctan\left(\frac{\epsilon_F^2+\Gamma^2-|M|^2}{2\Gamma|M|}\right)\right]. \tag{50}$$

One must be careful in taking the limit of this expression as $\Gamma \to 0$ as the argument of the arctangent when $\epsilon_F < |M|$ is in fact negative:

$$\lim_{\Gamma\to 0}\sigma_{yx}^{\mathrm{II}} = -\frac{e^2}{h}\frac{M}{2\pi|M|}\left[\frac{\pi}{2}+\frac{\pi}{2}\right] = -\mathrm{sgn}\,M\frac{e^2}{2h}. \tag{51}$$

We see that when the limit is correctly taken, the Hall conductivity within the mass gap is exactly quantized to half a conductance quantum, as expected. For completeness, we plot both contributions and their sum is Fig. 2.

## III. PERTURBATIVE EXPANSION OF TOTAL HALL CONDUCTIVITY

Figure 2 shows that when $\Gamma > 0$, $\sigma_{yx}^{\mathrm{I(a)}}$ within the gap becomes non-zero and $\sigma_{yx}^{\mathrm{II}}$ decreases from the quantized value. Despite these deviations from the Hermitian theory, the total Hall conductivity, $\sigma_{yx}$, appears to exhibit a large plateau of quantization when $\Gamma/|M| < 1$. To understand this behavior, we expand each contribution to the Hall conductivity in powers of $\Gamma$. We assume that $\epsilon_F < |M|$ since we are interested in the quantization of the Hall conductivity within the mass gap and consider the asymptotic expansion for $\arctan x$ (or equivalently the Taylor expansion of $\arctan\frac{1}{x}$):

$$\arctan x \sim \mathrm{sgn}\,x\frac{\pi}{2}-\frac{1}{x}+\frac{1}{3x^3}-\mathcal{O}(x^5). \tag{52}$$

Using this expression, we expand $\sigma_{yx}^{\mathrm{I(a)}}$ is powers of $\Gamma$:

$$\sigma_{yx}^{\mathrm{I(a)}} = \frac{e^2}{h}\frac{M}{\epsilon_F 2\pi}\left[\arctan\left(\frac{\Gamma^2+M^2-\epsilon_F^2}{2\epsilon_F\Gamma}\right)-\frac{\pi}{2}\right] \tag{53}$$

$$\lim_{\Gamma\to 0}\sigma_{yx}^{\mathrm{I(a)}} \sim \frac{e^2}{h}\frac{M}{\epsilon_F 2\pi}\left[\frac{\pi}{2}-\frac{2\epsilon_F\Gamma}{\Gamma^2+M^2-\epsilon_F^2}+\frac{8}{3}\frac{\epsilon_F^3\Gamma^3}{(\Gamma^2+M^2-\epsilon_F^2)^3}-\frac{\pi}{2}\right] \tag{54}$$

$$\sigma_{yx}^{\mathrm{I(a)}} \sim -\frac{e^2}{h}\left[\frac{1}{\pi}\frac{\Gamma M}{M^2-\epsilon_F^2}-\frac{4M}{3\pi}\frac{\epsilon_F^2\Gamma^3}{(M^2-\epsilon_F^2)^3}\right] \tag{55}$$

Similarly, $\sigma_{yx}^{\mathrm{II}}$ is expanded as

$$\sigma_{yx}^{\mathrm{II}} = \frac{e^2}{h}\frac{\operatorname{sgn} M}{2\pi}\left[\arctan\left(\frac{\epsilon_F^2+\Gamma^2-|M|^2}{2\Gamma|M|}\right)-\frac{\pi}{2}\right] \tag{56}$$

$$\lim_{\Gamma\to 0}\sigma_{yx}^{\mathrm{II}} \sim \frac{e^2}{h}\frac{M}{2\pi|M|}\left[-\frac{\pi}{2}-\frac{2\Gamma|M|}{\epsilon_F^2+\Gamma^2-|M|^2}+\frac{8}{3}\frac{\Gamma^3|M|^3}{(\epsilon_F^2+\Gamma^2-|M|^2)^3}-\frac{\pi}{2}\right] \tag{57}$$

$$\sigma_{yx}^{\mathrm{II}} \sim -\frac{e^2}{h}\left[\frac{\operatorname{sgn} M}{2}-\frac{1}{\pi}\frac{\Gamma M}{M^2-\epsilon_F^2}-\frac{4M}{3\pi}\frac{\Gamma^3 M^2}{(\epsilon_F^2-|M|^2)^3}\right] \tag{58}$$

From these approximations, we can see that the first order terms in $\sigma_{yx}^{\mathrm{I(a)}}$ and $\sigma_{yx}^{\mathrm{II}}$ exactly cancel:

$$\sigma_{yx}^{\mathrm{I(a)}} \sim -\frac{e^2}{h}\left[\qquad +\frac{1}{\pi}\frac{\Gamma M}{M^2-\epsilon_F^2}-\frac{4M}{3\pi}\frac{\epsilon_F^2\Gamma^3}{(M^2-\epsilon_F^2)^3}\right] \tag{59}$$

$$\sigma_{yx}^{\mathrm{II}} \sim -\frac{e^2}{h}\left[\frac{\operatorname{sgn} M}{2}-\frac{1}{\pi}\frac{\Gamma M}{M^2-\epsilon_F^2}-\frac{4M}{3\pi}\frac{\Gamma^3 M^2}{(\epsilon_F^2-|M|^2)^3}\right] \tag{60}$$

$$\sigma_{yx}^{\mathrm{tot}} \sim -\frac{e^2}{h}\left[\frac{\operatorname{sgn} M}{2}-\frac{4\Gamma^3 M}{3\pi}\frac{M^2+\epsilon_F^2}{(\epsilon_F^2-|M|^2)^3}\right]. \tag{61}$$

Therefore, the quantized plateau we observe in the total Hall conductivity in Fig. 2 is due to the fact that the leading order correction to the quantized Hall conductivity cubic in $\Gamma$. We note, however, that for any non-zero value of $\Gamma$, the Hall conductivity is no longer exactly quantized.

## IV. MAGNETIC IMPURITY SCATTERING

The second order term of the magnetic impurity scattering self-energy can be calculated as[8]

$$\Sigma_{\mathrm{eff}}^{(2)}(E) = \langle V G_0(E) V\rangle \tag{62}$$

$$= N_{\mathrm{imp}}\sum_{\mathbf{k}_1} U(\mathbf{k}-\mathbf{k}_1)G_0(E,\mathbf{k})U(\mathbf{k}_1-\mathbf{k}) \tag{63}$$

$$= \frac{N_{\mathrm{imp}}}{\mathcal{V}^2}\sum_{\mathbf{k}_1} u(\mathbf{k}-\mathbf{k}_1)G_0(E,\mathbf{k})u(\mathbf{k}_1-\mathbf{k}) \tag{64}$$

$$= n_{\mathrm{imp}}\frac{1}{\mathcal{V}}\sum_{\mathbf{k}_1} u_z\sigma_z G_0(E,\mathbf{k})u_z\sigma_z \tag{65}$$

$$= n_{\mathrm{imp}}u_z^2\int\frac{d\mathbf{k}}{(2\pi)^2}\,\sigma_z G_0^r(E,\mathbf{k})\sigma_z \tag{66}$$

$$= n_{\mathrm{imp}}u_z^2\sigma_0\int\frac{d\phi k\,dk}{(2\pi)^2}\,\frac{E+i0^+}{(E+i0^+)^2-\alpha^2k^2} \tag{67}$$

$$= \frac{n_{\mathrm{imp}}u_z^2}{2\pi}\sigma_0\int k\,dk\,\frac{1}{2}\left[\frac{1}{E-\alpha k+i0^+}+\frac{1}{E+\alpha k+i0^+}\right] \tag{68}$$

$$= \frac{n_{\mathrm{imp}}u_z^2}{2\pi}\sigma_0\int k\,dk\,\frac{1}{2}\left[\frac{1}{E-\alpha k}+\frac{1}{E+\alpha k}-i\pi\delta(E-\alpha k)-i\pi\delta(E+\alpha k)\right]. \tag{69}$$

Since the real part of this expression diverges, we adopt a Brillouin zone momentum cutoff $\Lambda_{\rm BZ} = \pi/a$, where $a$ is the lattice constant, to limit the calculation within the first Brillouin zone:[9]

$$\mathrm{Re}\,\Sigma^{(2)}_{\rm eff}(E) = \frac{n_{\rm imp}u_z^2}{4\pi}\sigma_0 \int_0^{\pi/a} dk \left[\frac{k}{E-\alpha k} + \frac{k}{E+\alpha k}\right] \tag{70}$$

$$= \frac{n_{\rm imp}u_z^2}{4\pi\alpha^2} E\left[\ln E^2 - \ln\left(E^2 - \frac{\alpha^2\pi^2}{a^2}\right)\right]\sigma_0 \tag{71}$$

$$= \frac{n_{\rm imp}u_z^2}{4\pi\alpha^2} E\ln\left(\frac{E^2}{E^2 - \frac{\alpha^2\pi^2}{a^2}}\right)\sigma_0. \tag{72}$$

This second-order effect in $u_z$ simply raises the on-site energy and does not change the qualitative physics of the problem.

The imaginary part of Eq. (69) gives the electrons a finite lifetime:

$$i\mathrm{Im}\,\Sigma^{(2)}_{\rm eff}(E) = -i\frac{n_{\rm imp}u_z^2}{4}\sigma_0 \int k\,dk\,\left[\delta(E-\alpha k) + \delta(E+\alpha k)\right] \tag{73}$$

$$= -i\frac{n_{\rm imp}u_z^2}{4|\alpha|}\sigma_0 \frac{E}{\alpha}\left[\theta\left(\frac{E}{\alpha}\right) - \theta\left(-\frac{E}{\alpha}\right)\right] \tag{74}$$

$$i\mathrm{Im}\,\Sigma^{(2)}_{\rm eff}(E) = -i\frac{n_{\rm imp}u_z^2}{4\alpha^2}|E|\sigma_0 \equiv -i\Gamma_{\rm imp}\,\sigma_0. \tag{75}$$

With the leading order contributions in the mass gap and the broadening in hand, we see that the ratio of the broadening to the mass gap,

$$\frac{\Gamma_{\rm imp}}{M_{\rm imp}} = \frac{|E|}{4\alpha^2}u_z \propto u_z, \tag{76}$$

is proportional to the perturbative parameter, $u_z$, which is taken to be much less than unity. As such, the Hall conductivity generated by the presence of magnetic dopants lies in the regime $\Gamma/M \ll 1$ where it deviates negligibly from the quantized value.

* tphilip3@illinois.edu


1. M. Pourfath, *The Non-Equilibrium Green's Function Method for Nanoscale Device Simulation*, Computational Microelectronics (Springer Vienna, Vienna, 2014).
2. M. P. L. Sancho, J. M. L. Sancho, and J. Rubio, J. Phys. F Met. Phys. **14**, 1205 (1984).
3. M. P. L. Sancho, J. M. L. Sancho, J. M. L. Sancho, and J. Rubio, J. Phys. F Met. Phys. **15**, 851 (1985).
4. N. A. Sinitsyn, A. H. MacDonald, T. Jungwirth, V. K. Dugaev, and J. Sinova, Phys. Rev. B **75**, 045315 (2007), arXiv:0608682 [cond-mat].
5. T. S. Nunner, N. A. Sinitsyn, M. F. Borunda, V. K. Dugaev, A. A. Kovalev, A. Abanov, C. Timm, T. Jungwirth, J.-i. Inoue, A. H. MacDonald, and J. Sinova, Phys. Rev. B **76**, 235312 (2007), arXiv:0502386 [cond-mat].
6. P. Streda, J. Phys. C Solid State Phys. **15**, 717 (1982).
7. C. Chang, J. Zhang, X. Feng, J. Shen, Z. Zhang, M. Guo, K. Li, Y. Ou, P. Wei, L.-L. Wang, Z.-Q. Ji, Y. Feng, S. Ji, X. Chen, J. Jia, X. Dai, Z. Fang, S.-C. Zhang, K. He, Y. Wang, L. Lu, X.-C. Ma, and Q.-K. Xue, Science **340**, 167 (2013).
8. H. Bruus and K. Flensberg, *Many-Body Quantum Theory in Condensed Matter Physics: An Introduction* (Oxford University Press, Oxford, 2004).
9. A. Sakai and H. Kohno, Phys. Rev. B **89**, 165307 (2014), arXiv:arXiv:1309.4195v1.
10. C. W. Groth, M. Wimmer, A. R. Akhmerov, J. Tworzydło, and C. W. Beenakker, Phys. Rev. Lett. **103**, 1 (2009), arXiv:0908.0881.
